# Supplementary material for: Automatic differential analysis of NMR experiments in complex samples
Source: arXiv:1707.08805 source file (2017-07-27)

Supporting Information

# Automatic differential analysis of NMR experiments in complex samples

Laure Margueritte, Petar Markov, Lionel Chiron, Jean-Philippe Starck, Catherine Vonthron-Sénécheau, Mélanie Bourjot, Marc-André Delsuc*

**Spectra of sample 1 :**

S1 - $^{1}$H NMR spectrum (MeOD, 700 MHz)

S2 - COSY spectrum (MeOD, 700 MHz)

S3 - TOCSY spectrum (MeOD, 700 MHz)

S4 - HSQC spectrum (MeOD, 700 MHz)

S5 - HMBC spectrum (MeOD, 700 MHz)

S6 - DOSY spectrum (MeOD, 700 MHz)

**Spectra of sample 2 :**

S7 - $^{1}$H NMR spectrum (MeOD, 700 MHz)

S8 - COSY spectrum (MeOD, 700 MHz)

S9 - TOCSY spectrum (MeOD, 700 MHz)

S10 - HSQC spectrum (MeOD, 700 MHz)

S11 - HMBC spectrum (MeOD, 700 MHz)

S12 - DOSY spectrum (MeOD, 700 MHz)

**Spectra of sample 3 :**

S13 - $^{1}$H NMR spectrum (MeOD, 700 MHz)

S14 - COSY spectrum (MeOD, 700 MHz)

S15 - TOCSY spectrum (MeOD, 700 MHz)

S16 - HSQC spectrum (MeOD, 700 MHz)

S17 - HMBC spectrum (MeOD, 700 MHz)

S18 - DOSY spectrum (MeOD, 700 MHz)

**Spectra of sample 4 :**

S19 - $^{1}$H NMR spectrum (MeOD, 700 MHz)

S20 - COSY spectrum (MeOD, 700 MHz)

S21 - TOCSY spectrum (MeOD, 700 MHz)

S22 - HSQC spectrum (MeOD, 700 MHz)

S23 - HMBC spectrum (MeOD, 700 MHz)

S24 - DOSY spectrum (MeOD, 700 MHz)

**Spectra of sample 5 :**

S25 - $^{1}H$ NMR spectrum (MeOD, 700 MHz)

S26 - COSY spectrum (MeOD, 700 MHz)

S27 - TOCSY spectrum (MeOD, 700 MHz)

S28 - HSQC spectrum (MeOD, 700 MHz)

S29 - HMBC spectrum (MeOD, 700 MHz)

S30 - DOSY spectrum (MeOD, 700 MHz)

S1 - $^{1}$H NMR spectrum (MeOD, 700 MHz)

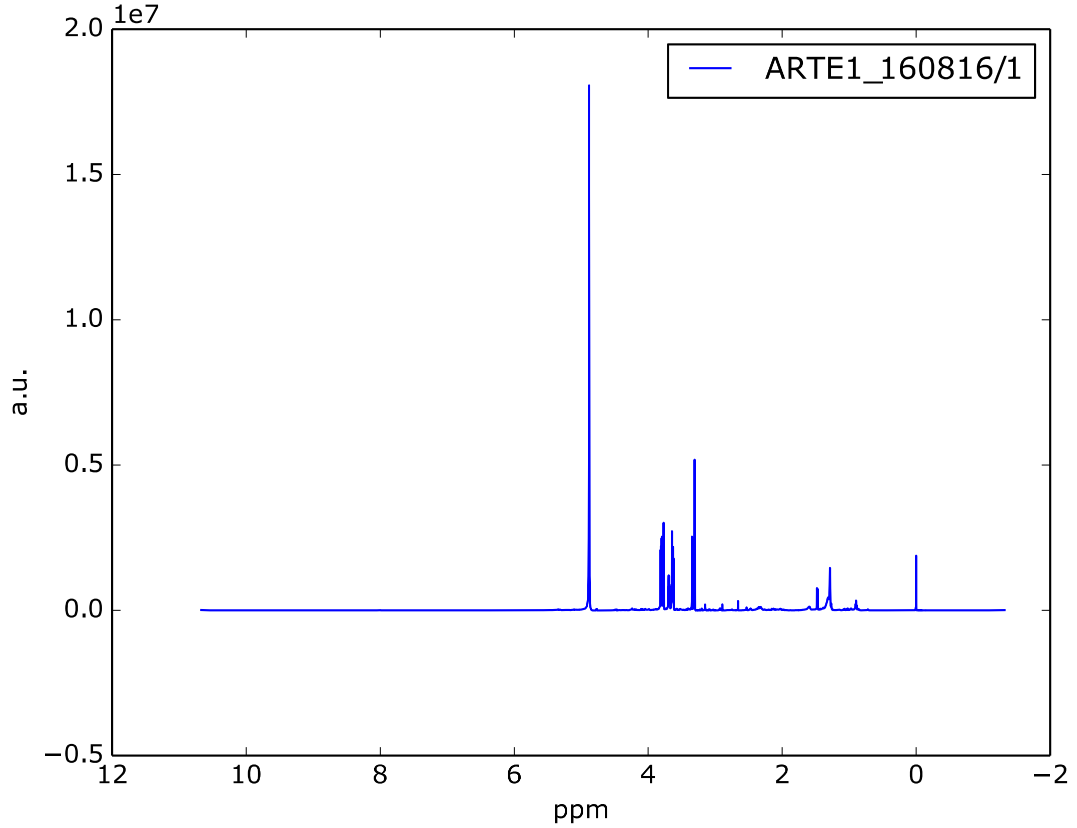


S2 - COSY spectrum (MeOD, 700 MHz)

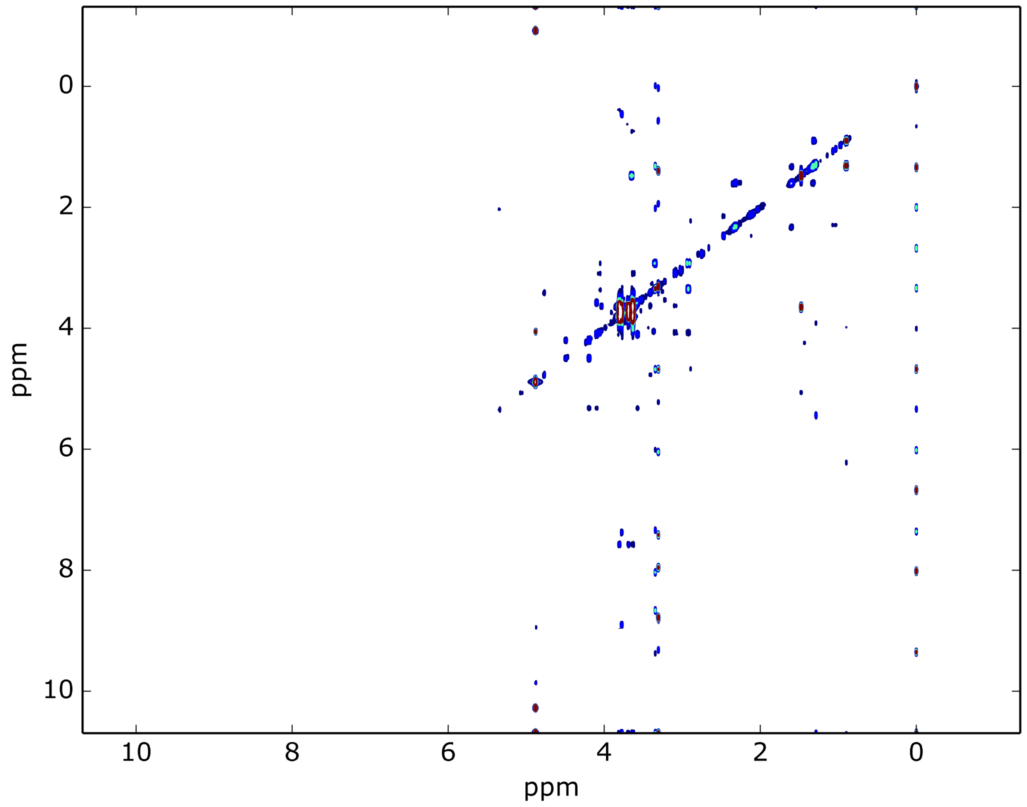

S3 - TOCSY spectrum (MeOD, 700 MHz)

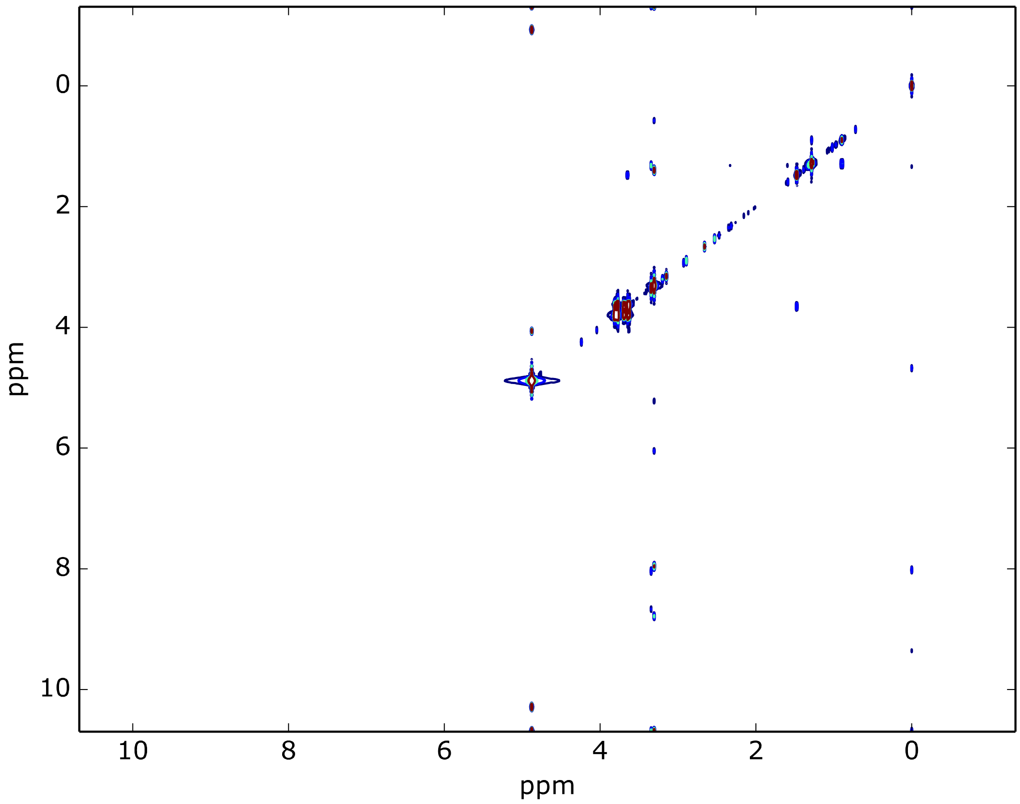


S4 - HSQC spectrum (MeOD, 700 MHz)

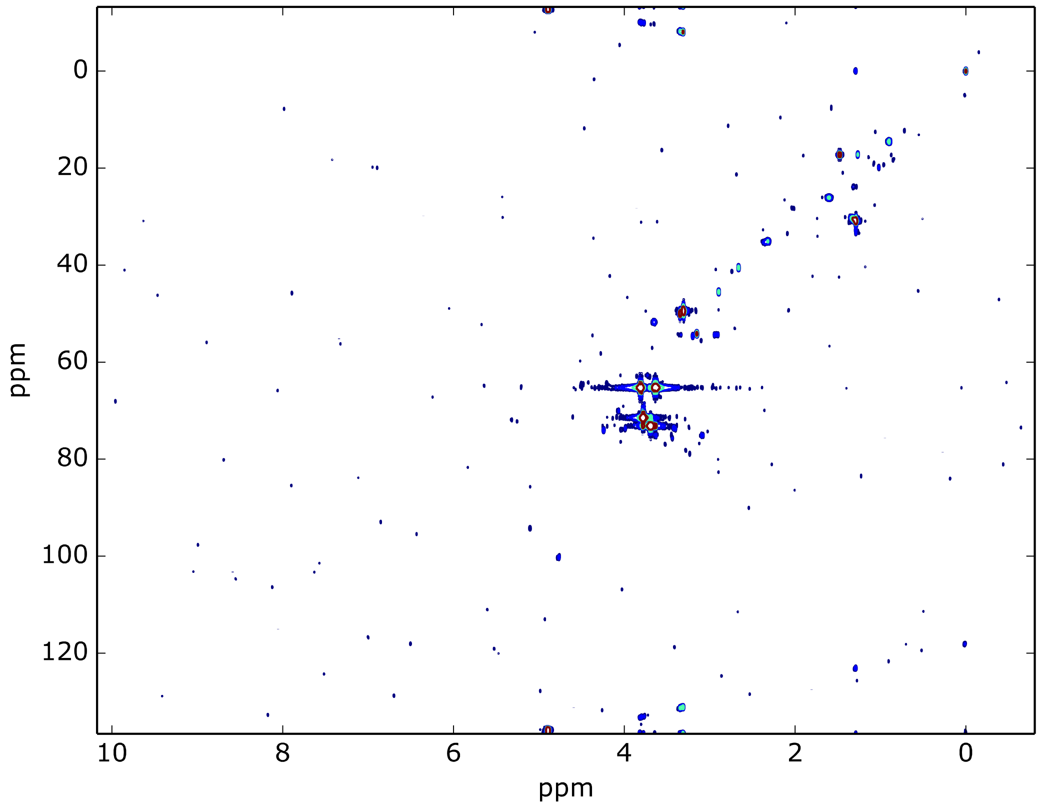

S5 - HMBC spectrum (MeOD, 700 MHz)

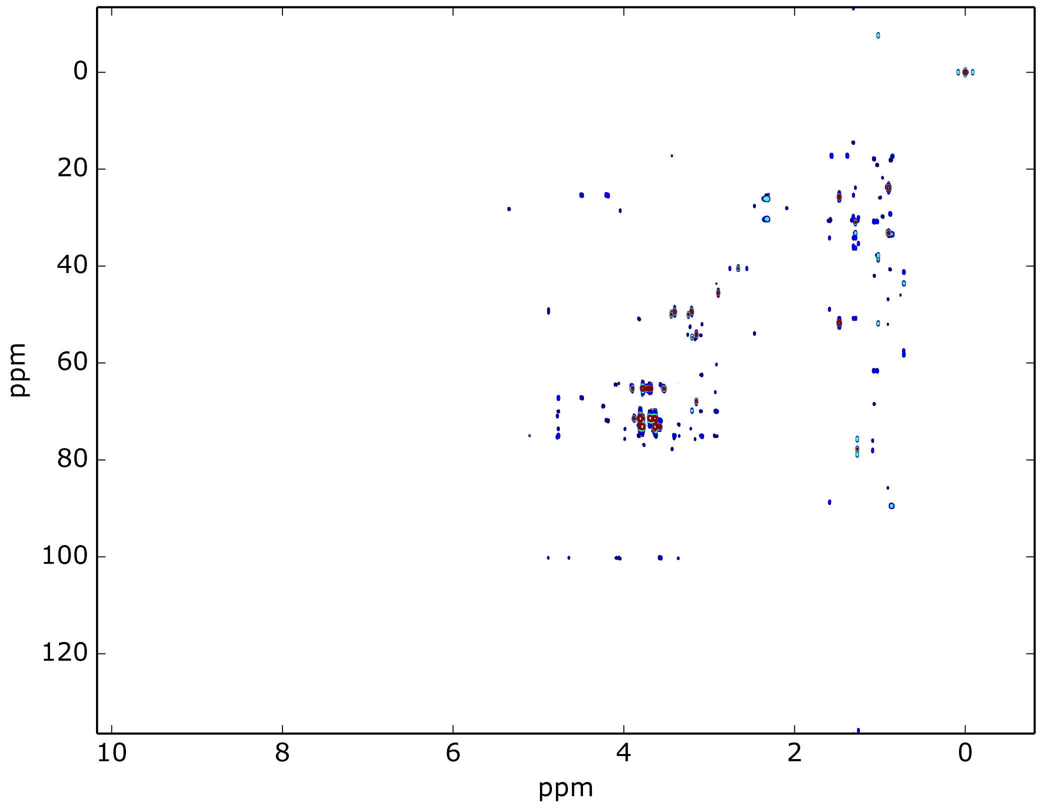


S6 - DOSY spectrum (MeOD, 700 MHz)

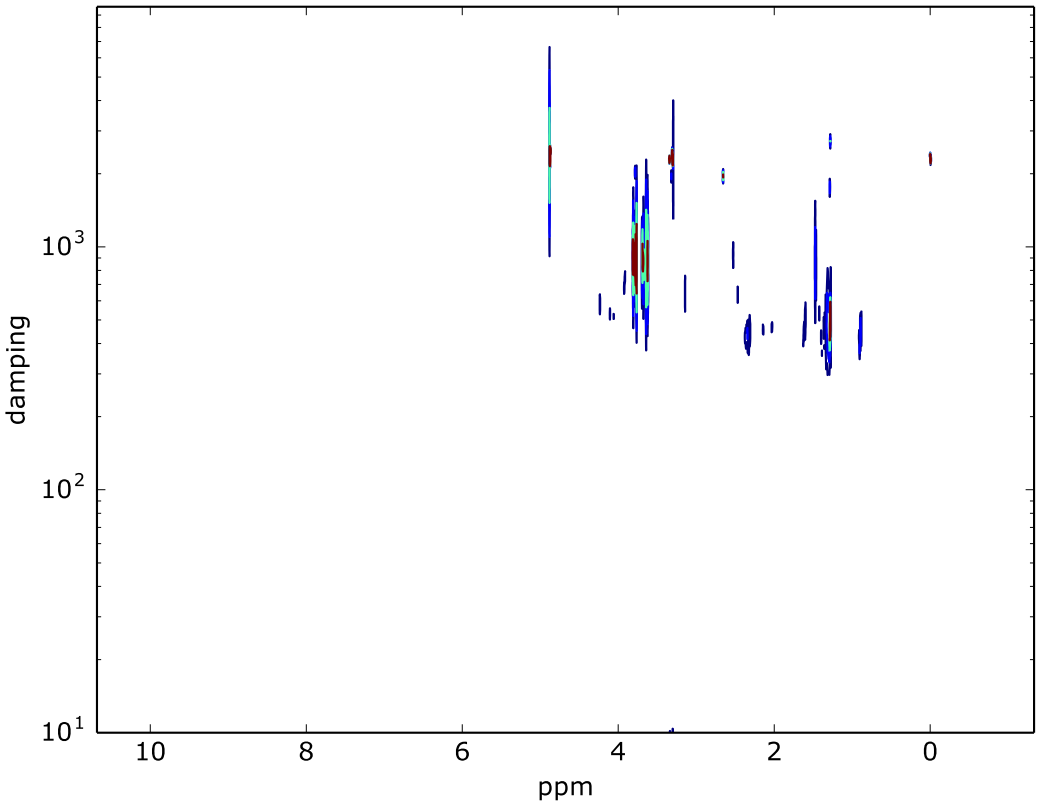

S7 - $^{1}$H NMR spectrum (MeOD, 700 MHz)

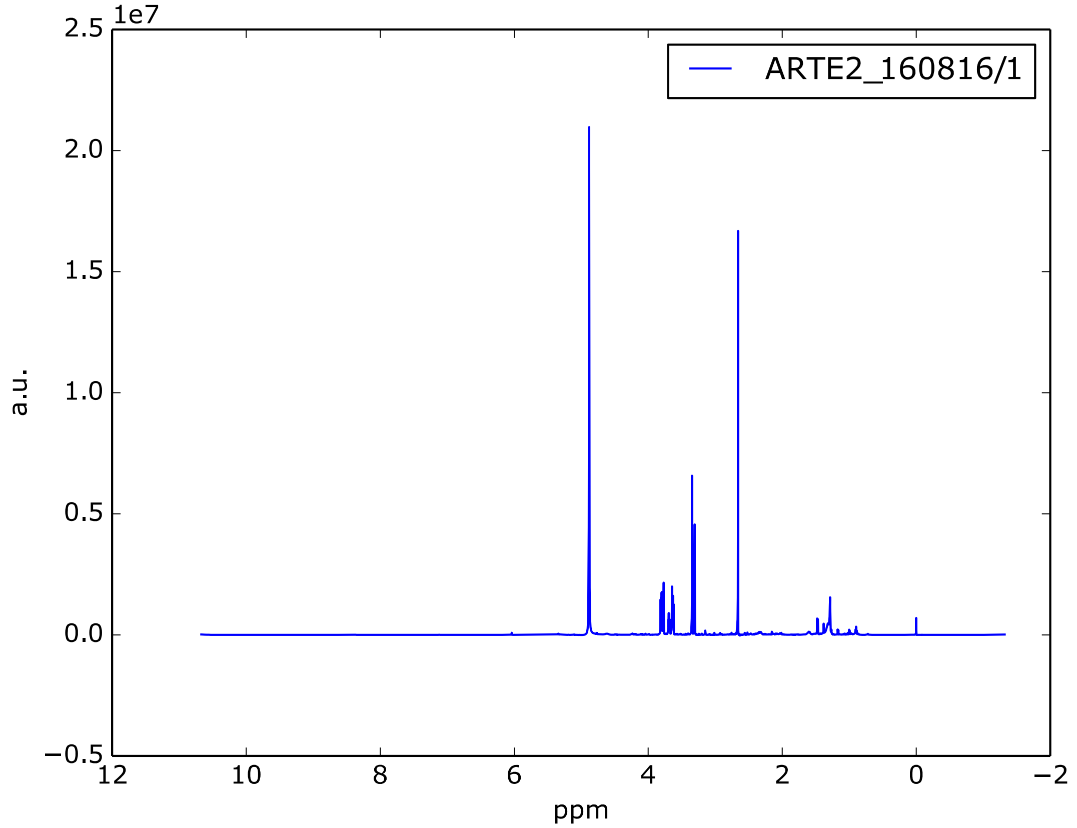


S8 - COSY spectrum (MeOD, 700 MHz)

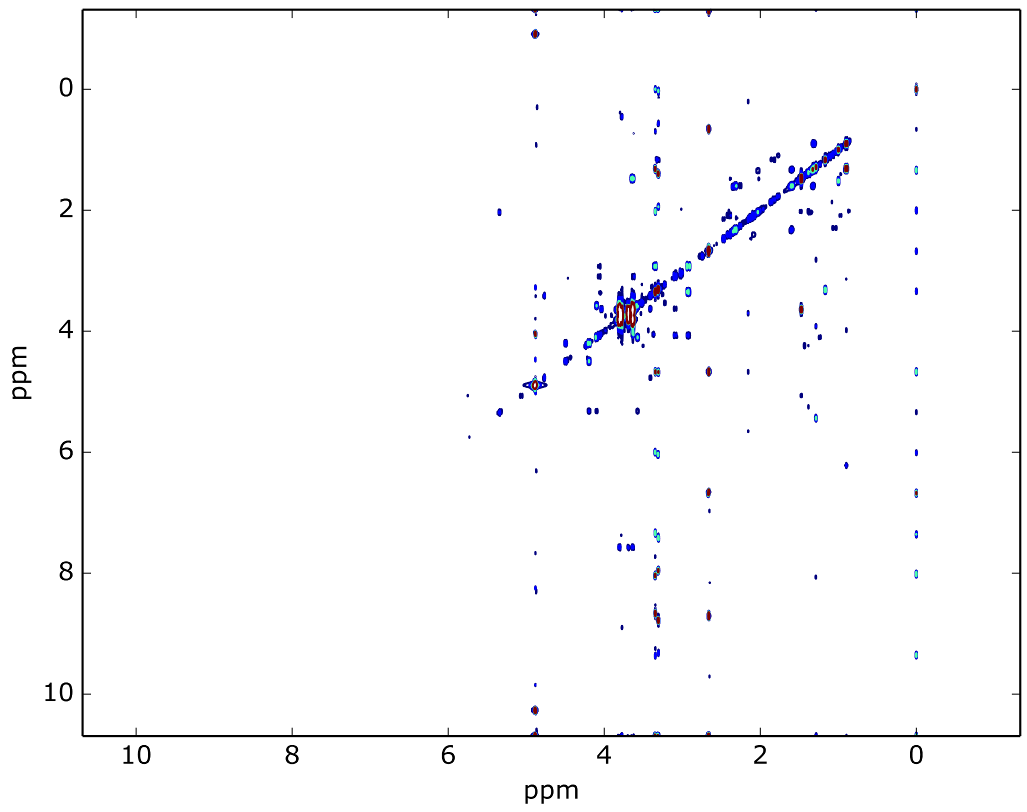

S9 - TOCSY spectrum (MeOD, 700 MHz)

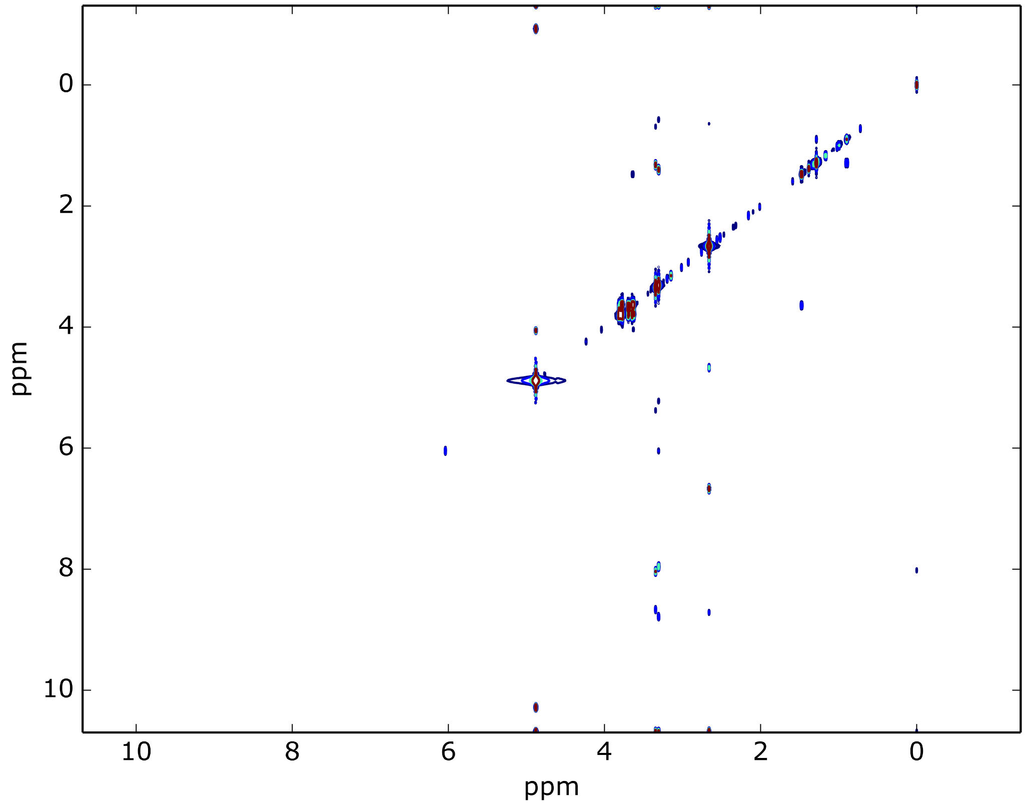


S10 - HSQC spectrum (MeOD, 700 MHz)

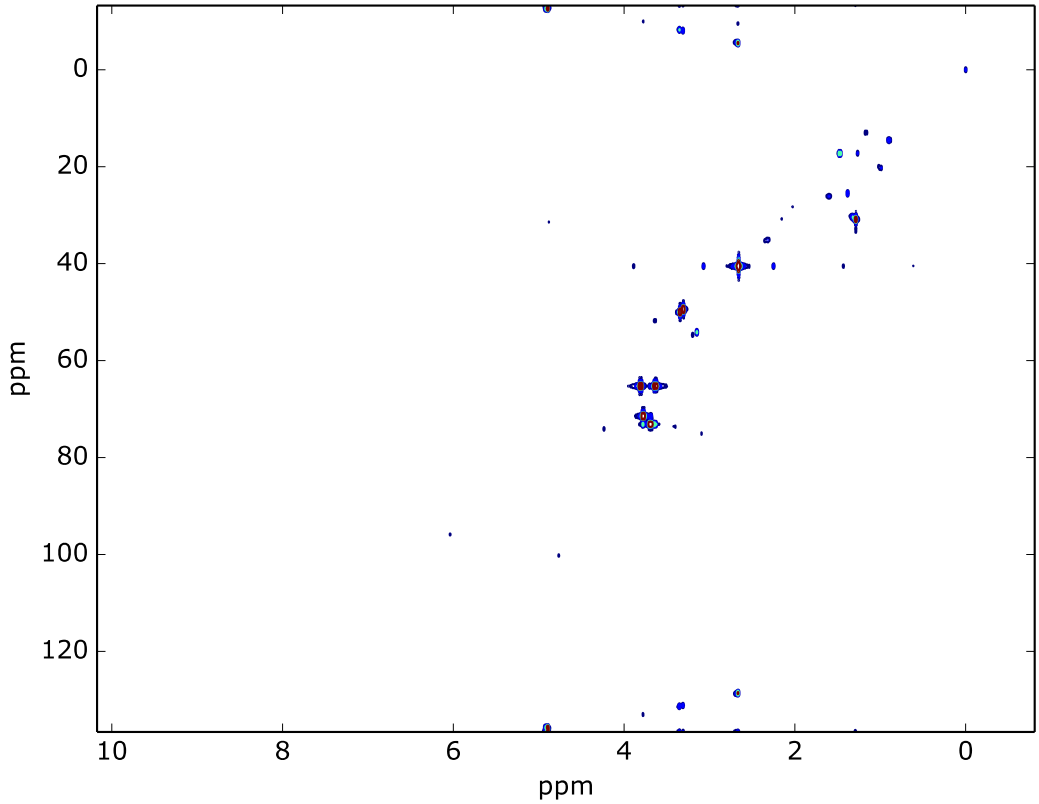

S11 - HMBC spectrum (MeOD, 700 MHz)

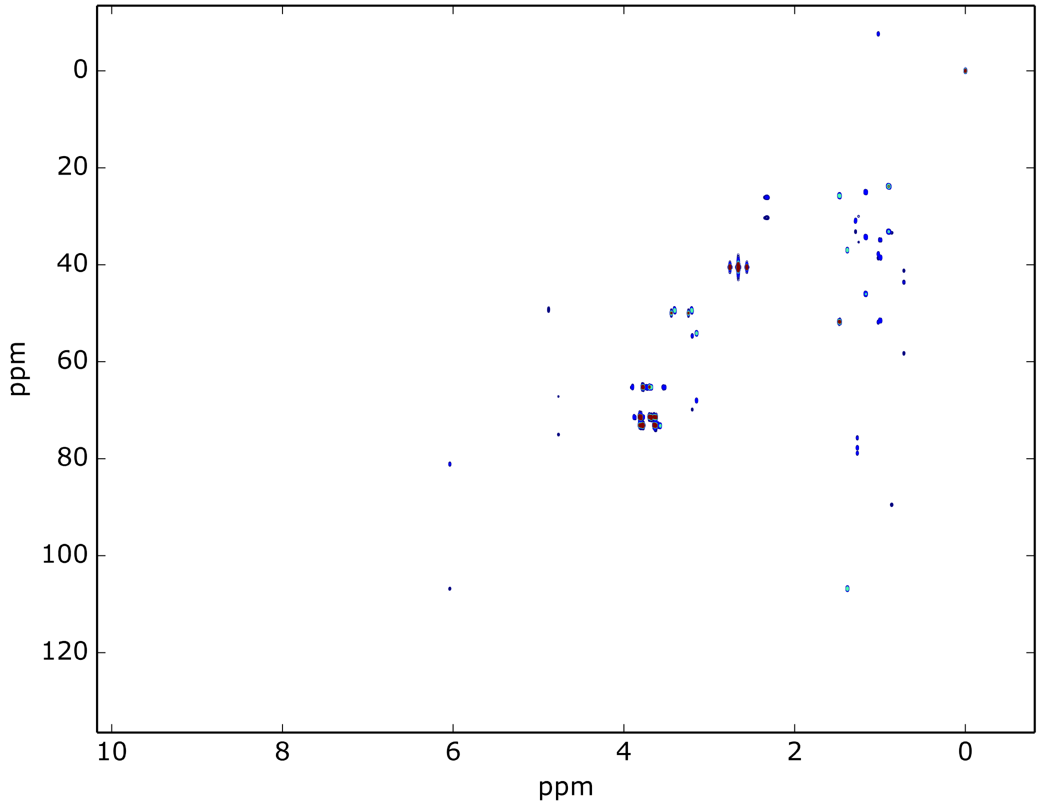


S12 - DOSY spectrum (MeOD, 700 MHz)

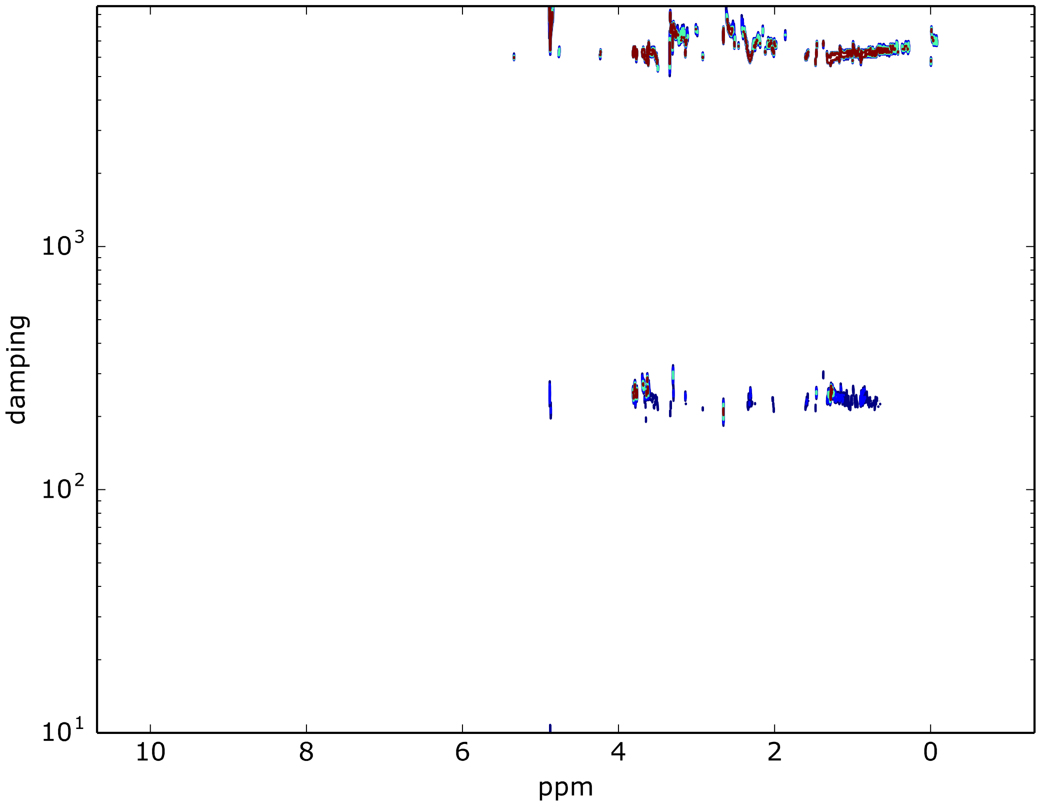

S13 - $^{1}$H NMR spectrum (MeOD, 700 MHz)

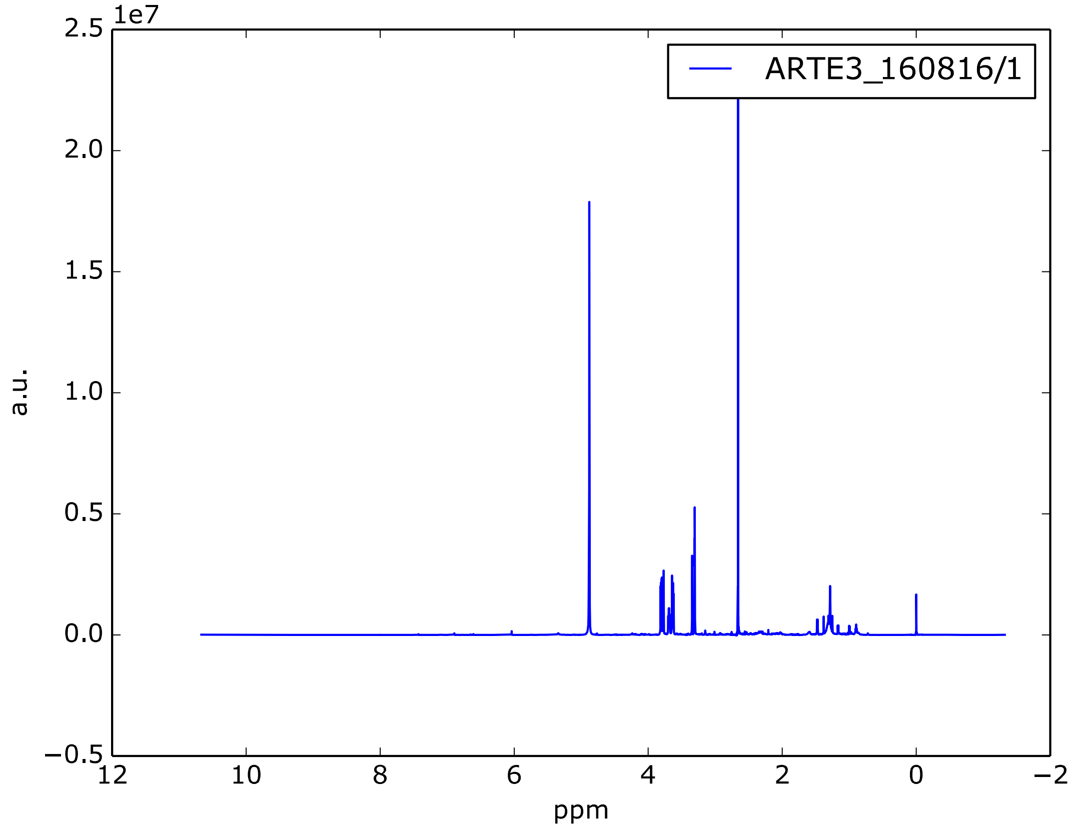


S14 - COSY spectrum (MeOD, 700 MHz)

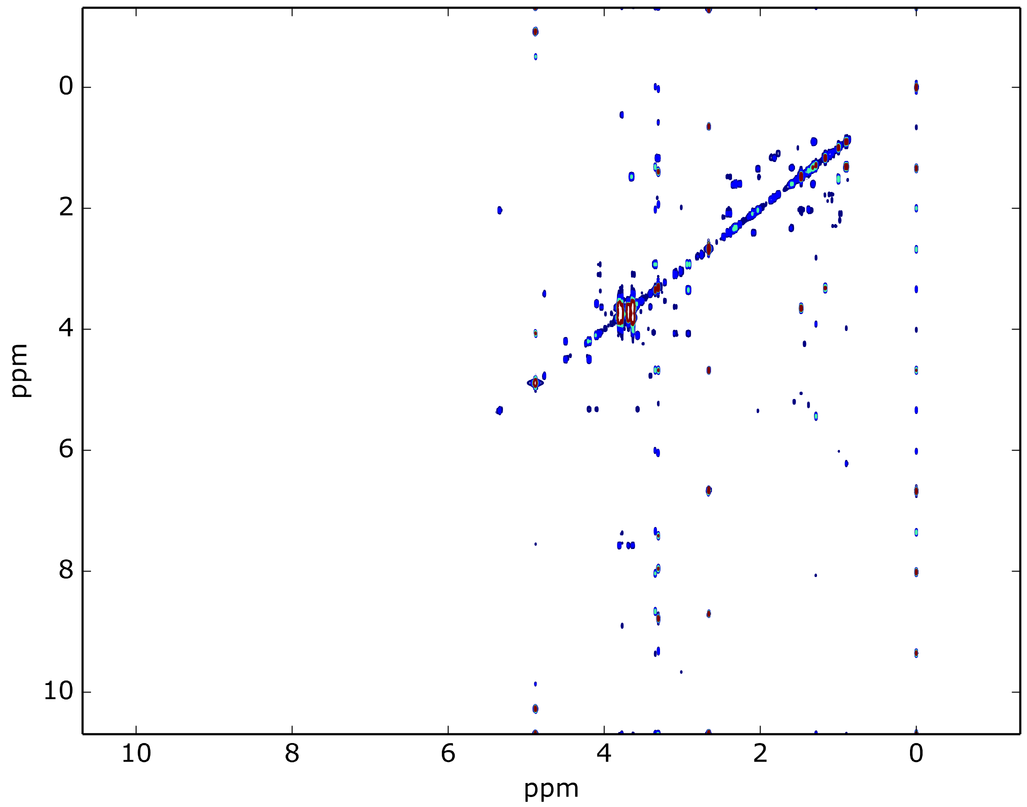

S15 - TOCSY spectrum (MeOD, 700 MHz)

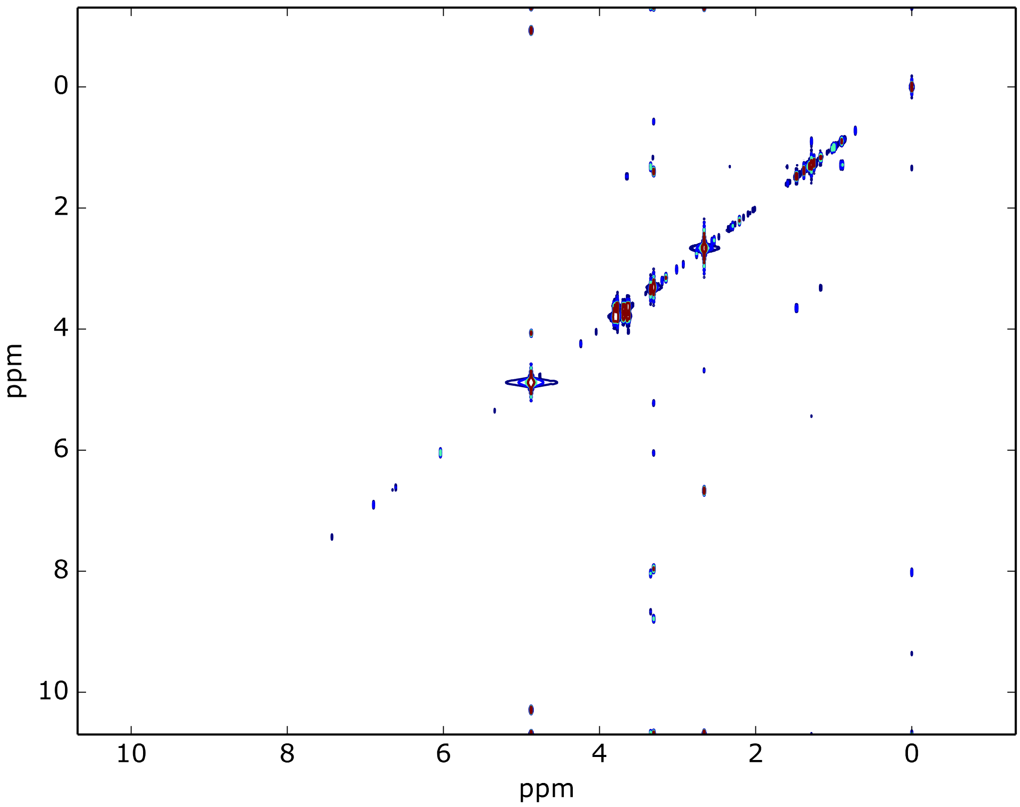


S16 - HSQC spectrum (MeOD, 700 MHz)

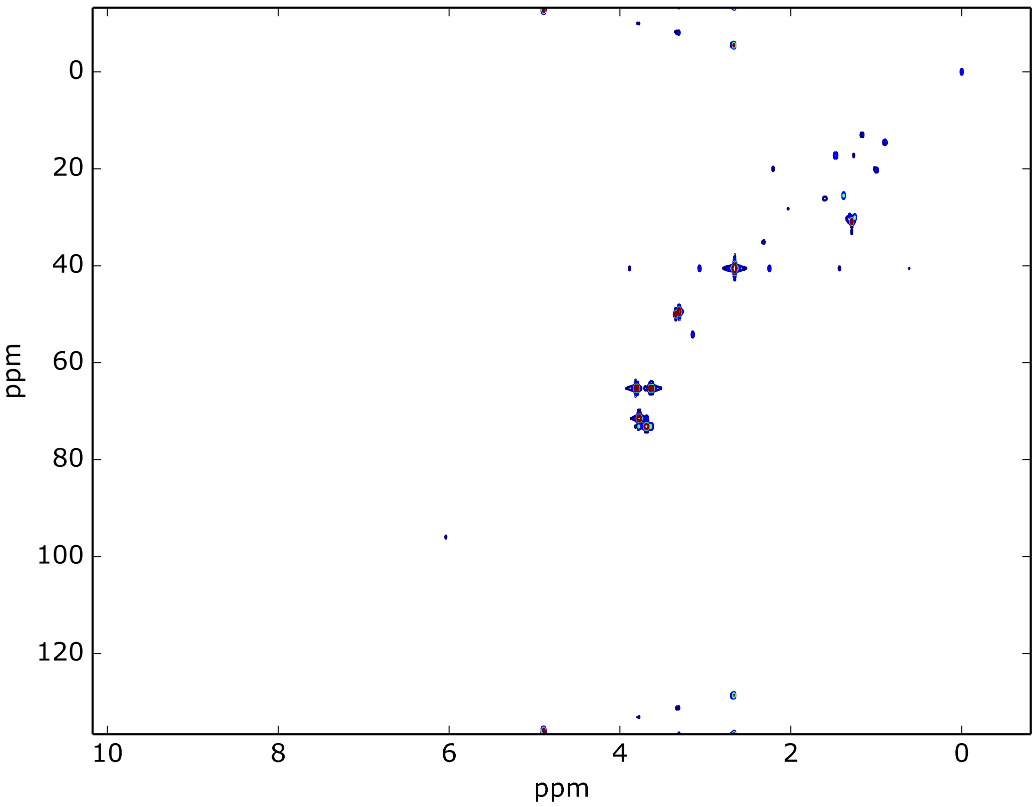

S17 - HMBC spectrum (MeOD, 700 MHz)

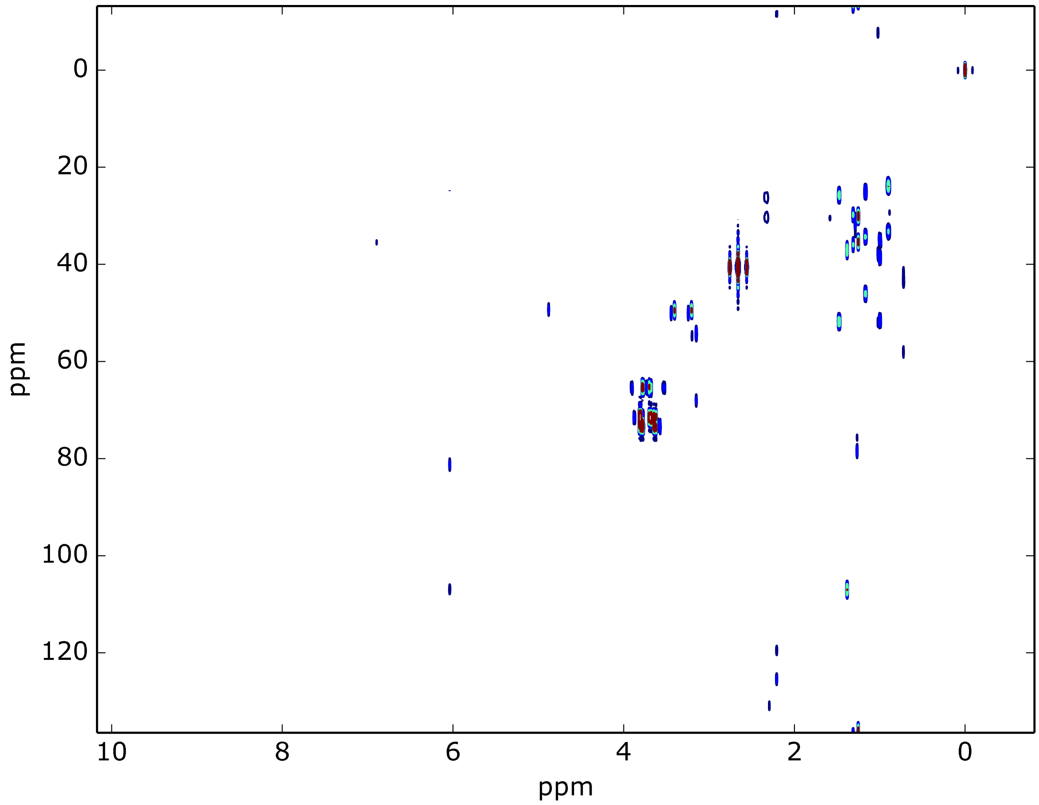


S18 - DOSY spectrum (MeOD, 700 MHz)

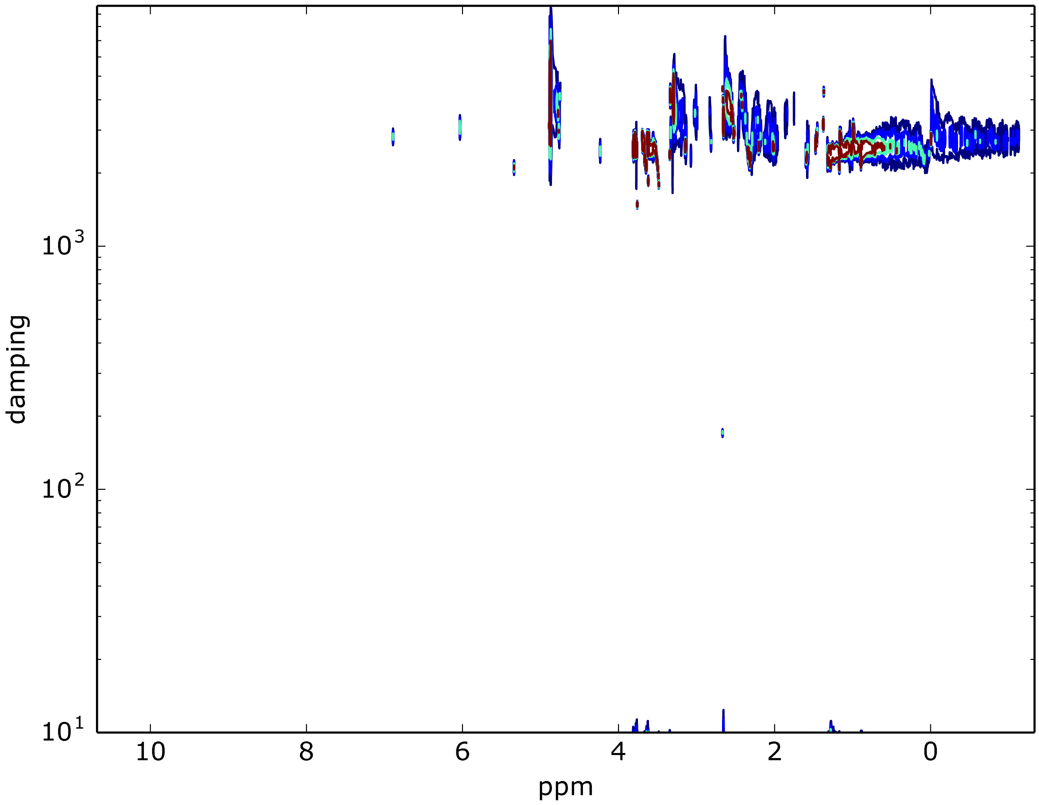

S19 - $^{1}$H NMR spectrum (MeOD, 700 MHz)

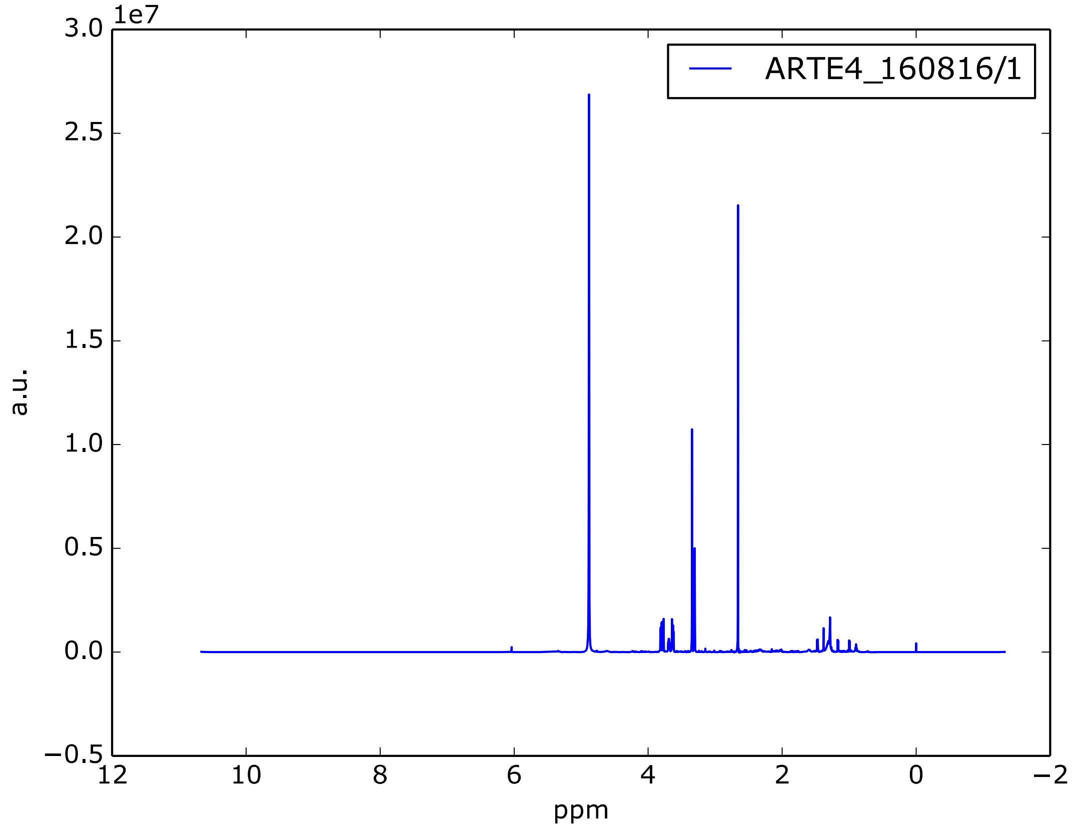


S20 - COSY spectrum (MeOD, 700 MHz)

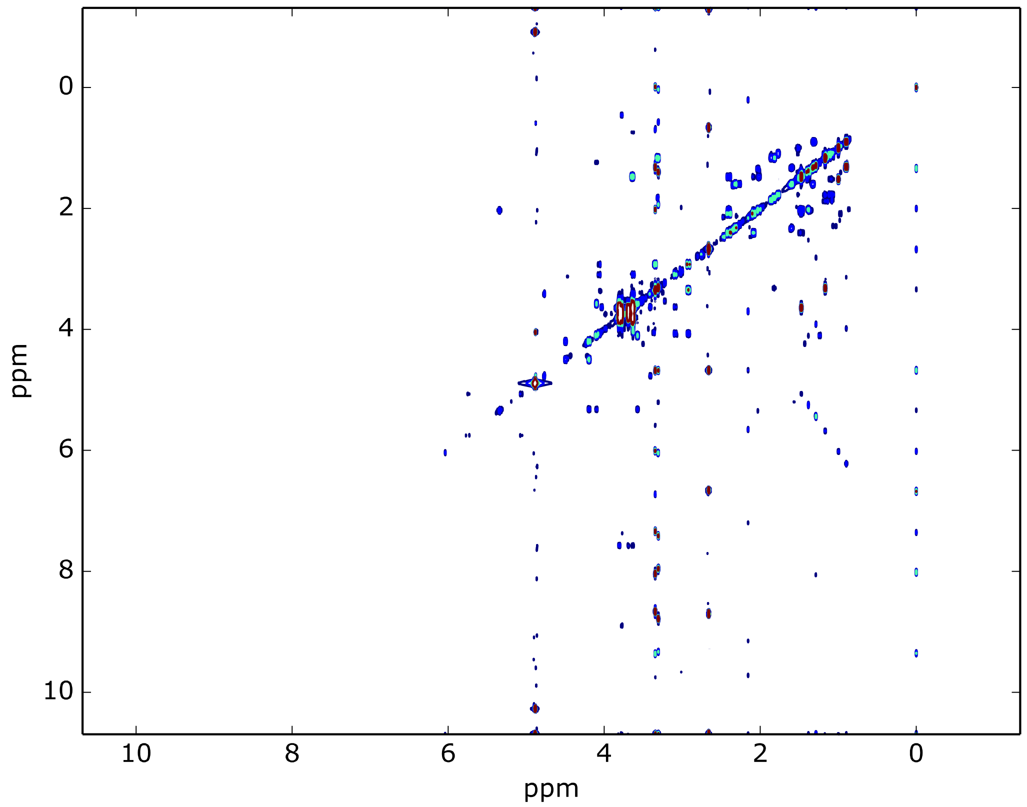

S21 - TOCSY spectrum (MeOD, 700 MHz)

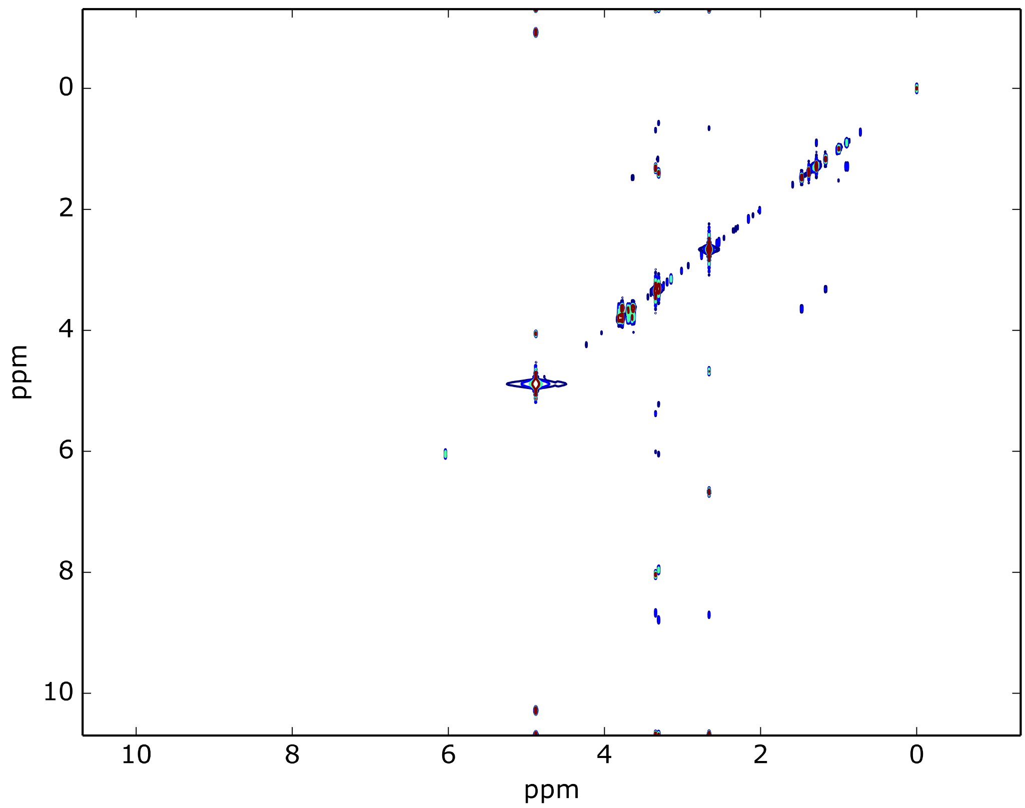


S22 - HSQC spectrum (MeOD, 700 MHz)

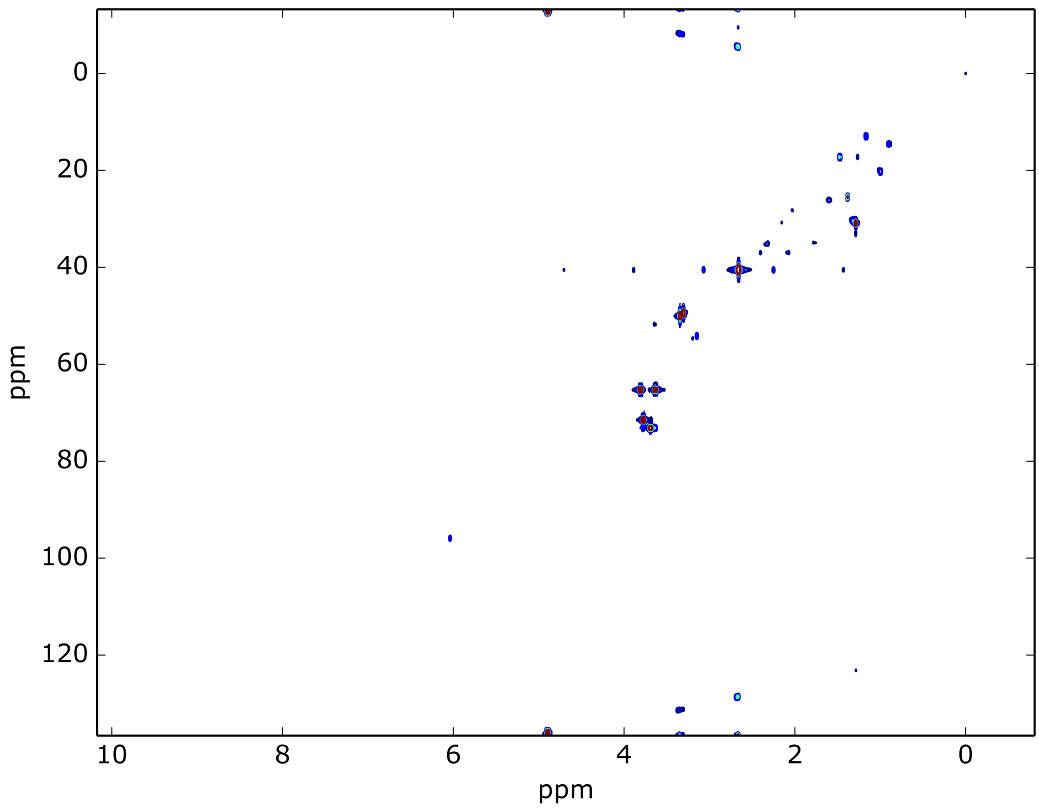

S23 - HMBC spectrum (MeOD, 700 MHz)

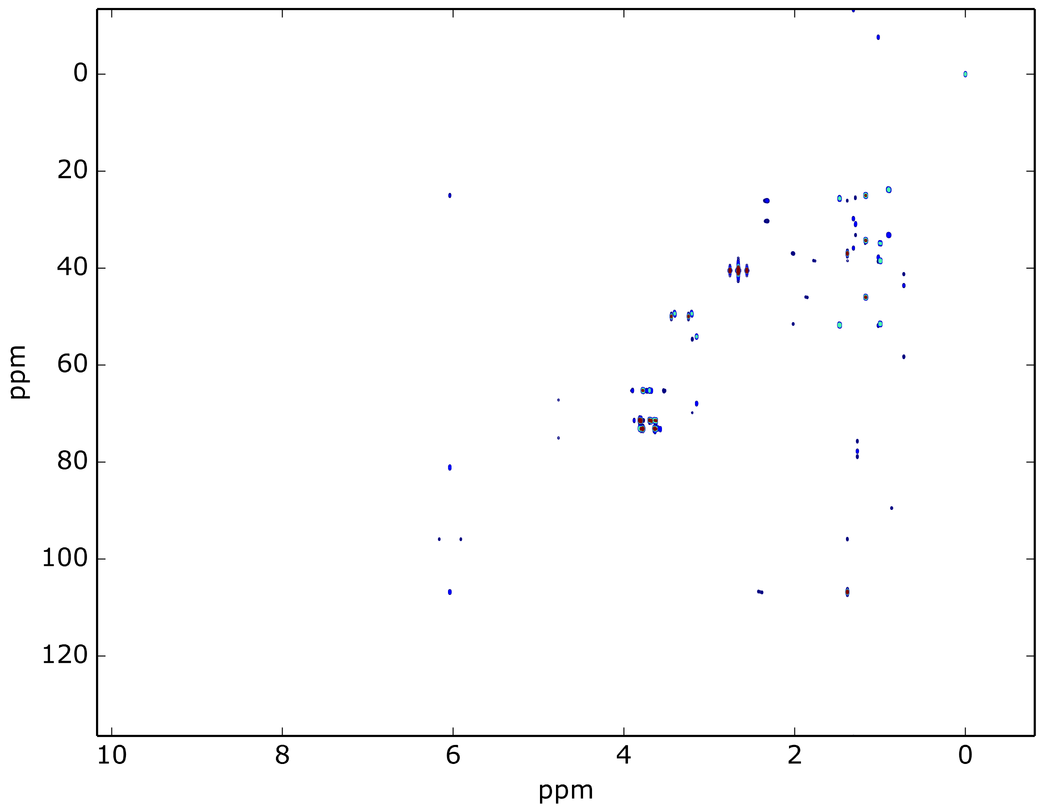


S24 - DOSY spectrum (MeOD, 700 MHz)

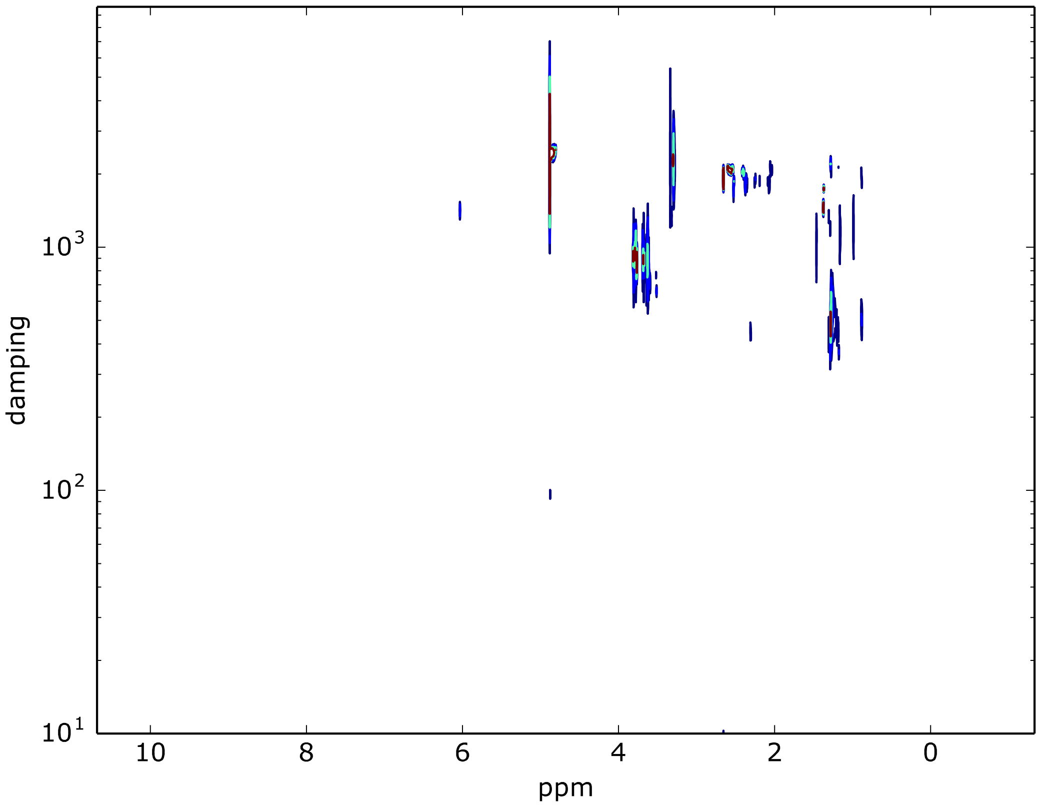

S25 - $^{1}$H NMR spectrum (MeOD, 700 MHz)

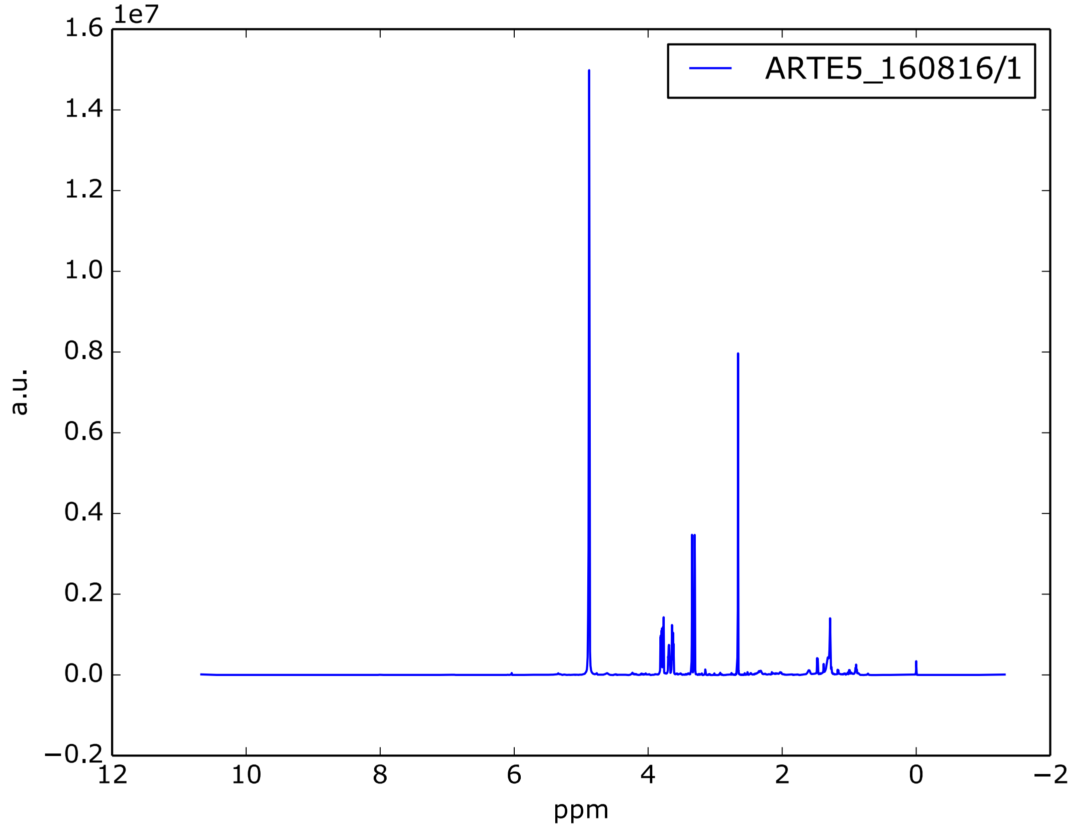


S26 - COSY spectrum (MeOD, 700 MHz)

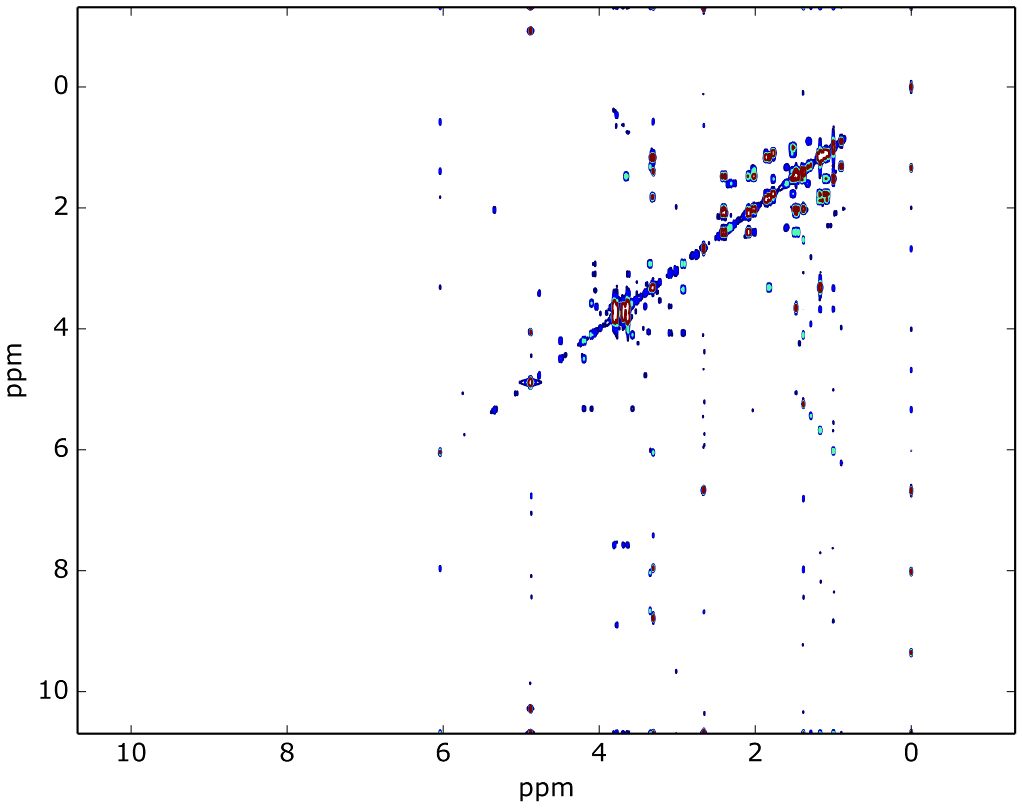

S27 - TOCSY spectrum (MeOD, 700 MHz)

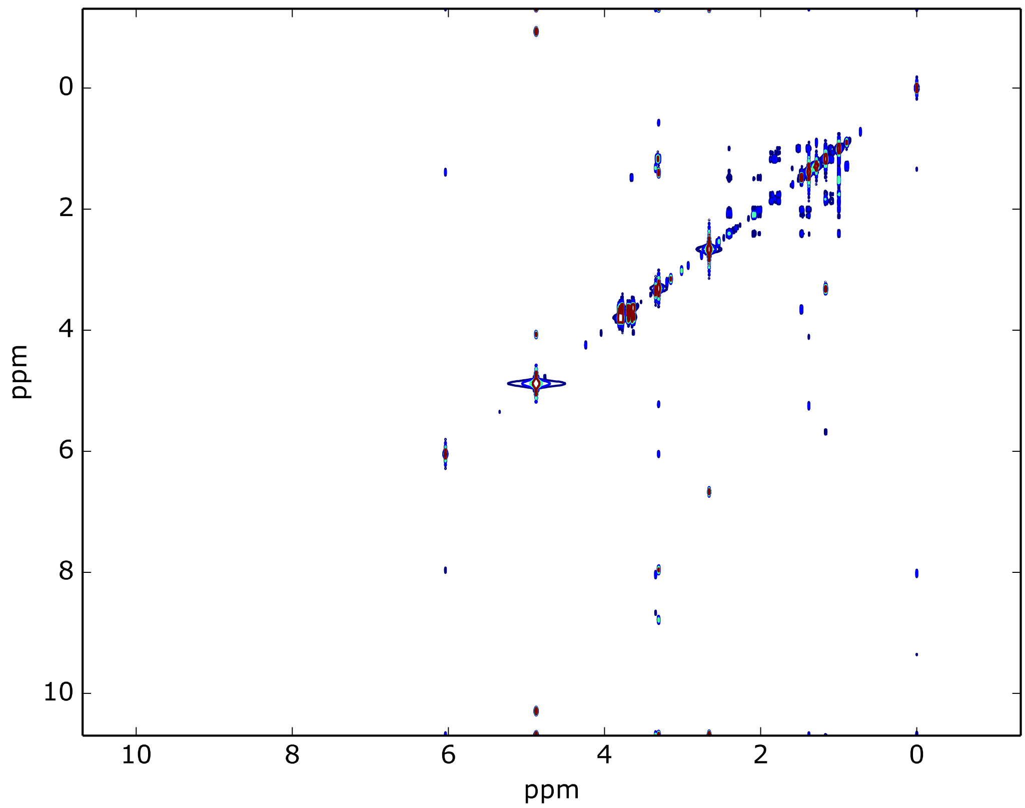


S28 - HSQC spectrum (MeOD, 700 MHz)

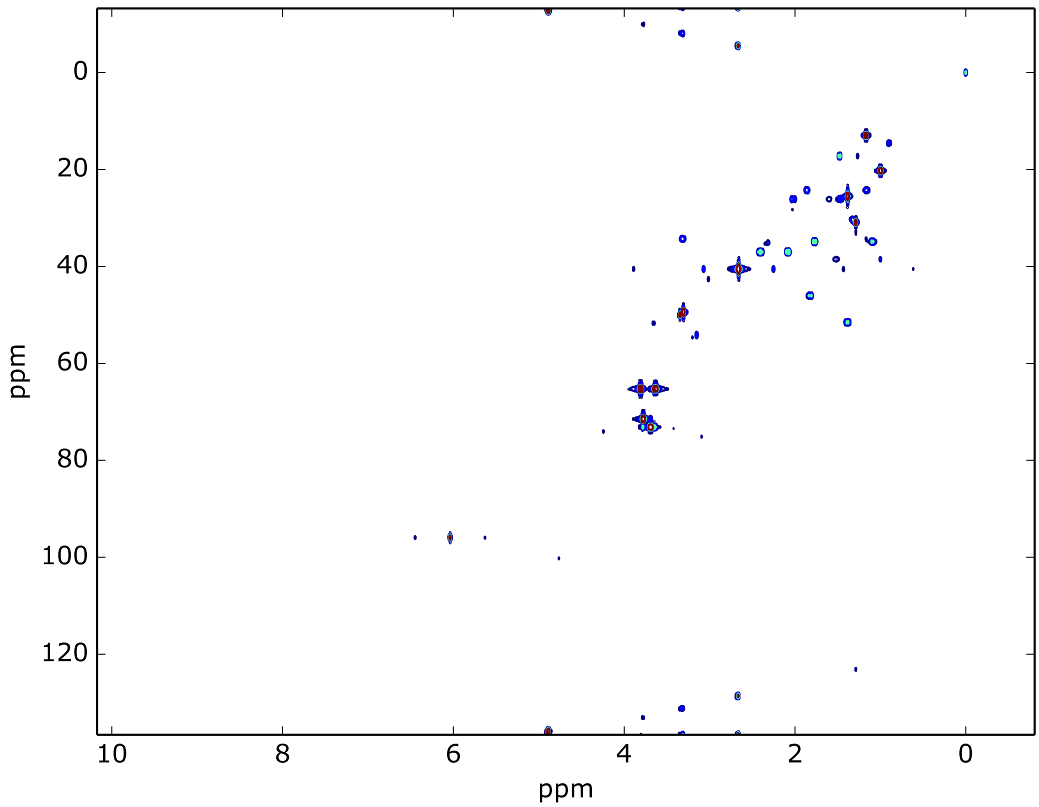

S29 - HMBC spectrum (MeOD, 700 MHz)

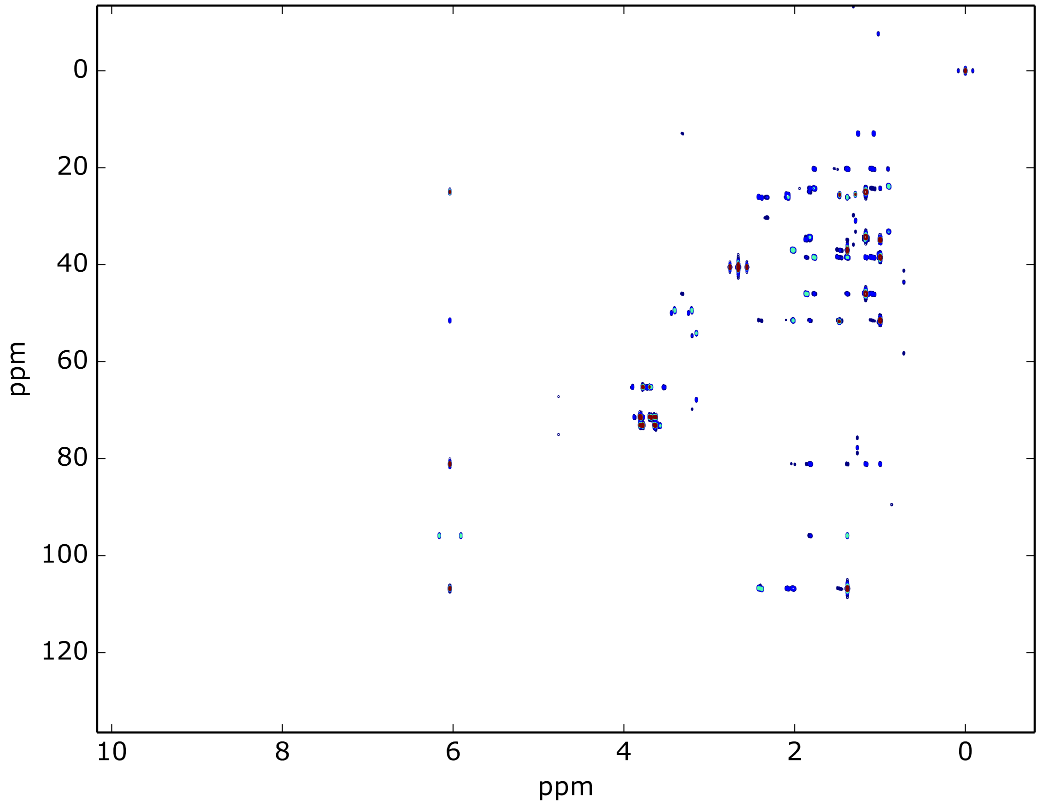


S30 - DOSY spectrum (MeOD, 700 MHz)

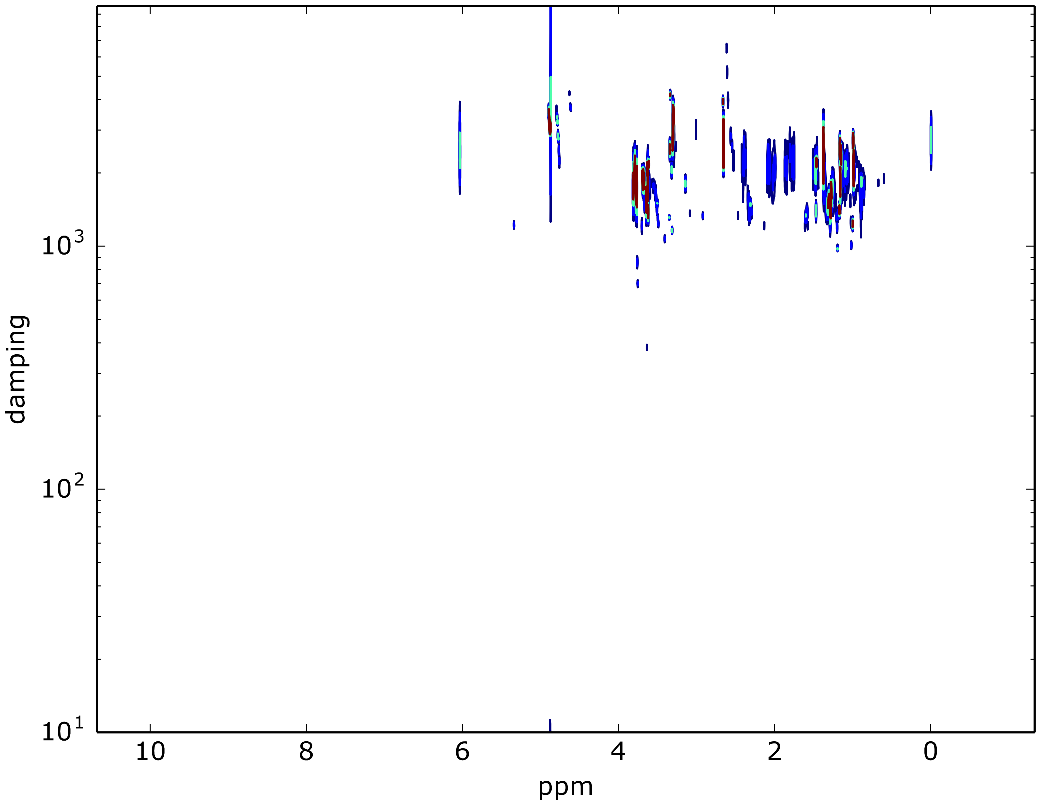

Supplement: Supplementary file 1 [file SI1.pdf]
